# Supplementary material for: Distantly-Supervised Evidence Retrieval Enables Question Answering without Evidence Annotation
Source: arXiv:2110.04889 source file (2021-10-10)
Supplement: Supplementary file 1 [file appendix.tex]

\appendix
\label{sec:app-impl}
